# Supplementary material for: Understanding Interfacial Ice Premelting: Structure, Adhesion and Nucleation
Source: arXiv:2410.21893 source file (2024-10-29)
Supplement: Supplementary file 1 [file supp-materials.pdf]

# Supporting Materials: Understanding Interfacial Ice Premelting: Structure, Adhesion and Nucleation

Łukasz Baran,[*,†] Pablo Llombart,[‡] and Luis G. MacDowell[*,¶]

†*Department of Theoretical Chemistry, Institute of Chemical Sciences, Faculty of Chemistry, Maria Curie-Sklodowska University in Lublin, Lublin, Poland.*

‡*Departamento de Física Teórica de la Materia Condensada, Instituto Nicolás Cabrera, Universidad Autńoma de Madrid, Madrid 28049, Spain*

¶*Departamento de Química Física, Facultad de Ciencias Químicas, Universidad Complutense, Madrid, 28040, Spain.*

E-mail: lukasz.baran@mail.umcs.pl; lgmac@quim.ucm.es

# Estimation of melting pressure

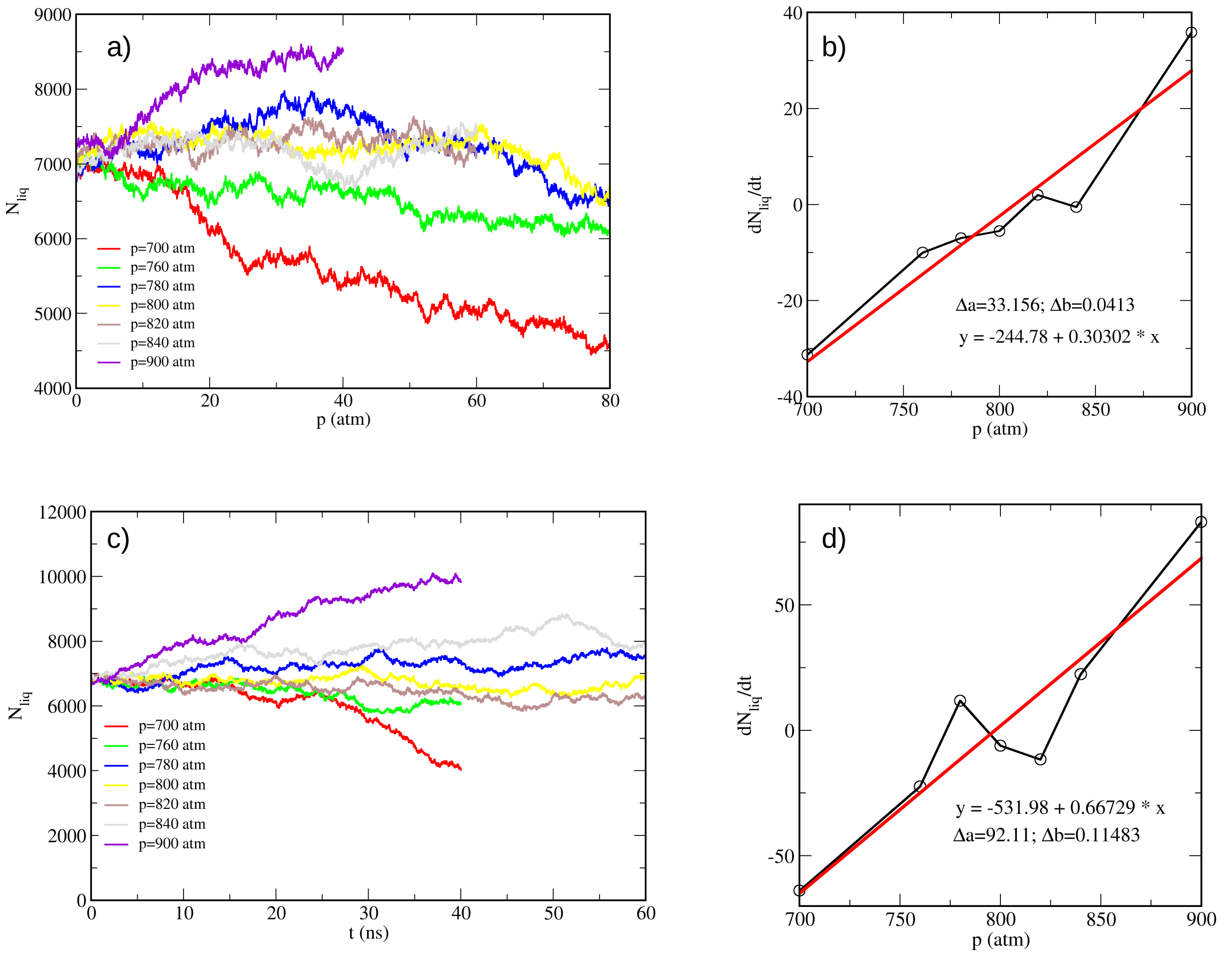


Figure S1: Relation of the number of liquid molecules with respect to time for basal (0001) (a) and secondary prism ($\bar{1}2\bar{1}0$) (c) faces. Melting/freezing rate for the basal (b) and the secondary prism faces (d). The linear regression is shown as a red solid line in parts (b, d).

To determine the melting pressure of ice Ih at $T = 262$ K we have employed a direct coexistence method.[1,2] As briefly mentioned in the main text, two phases at coexistence are brought together across an interface and the rate of change of the number of liquid/solid molecules is monitored during the simulations in the $Np_{\perp}AT$ ensemble.

Even though the melting point should not depend on the exposed facet, the kinetics of the process can. For this reason, we have studied two cases where a solid-liquid interface has been created at (i) the basal (0001) and (ii) secondary prism ($\bar{1}2\bar{1}0$) faces of ice Ih. In

fact, secondary prism facet (pII) has been selected because it exhibits the fastest kinetics of the melting process[3] in comparison to the basal face. It is due to the fact that basal facet is a "smooth" surface that melts/freezes epitaxially (layer by layer) and each of such layering transitions has its own energy barrier that has to be overcome, requiring much larger simulation times. On the other hand, the secondary prism is "rough" and therefore, should melt/freeze in the entire volume. Moreover, it has been reported that competing polymorphic form of ice Ic can be formed on the basal face, forming the so-called stacking hybrids of interwoven cubic and hexagonal ices, which is not the case for the secondary prism face. This can also be a reason for slower ice growth kinetics and has been demonstrated that such behavior is highly dependent on the thermodynamic conditions such as the degree of supercooling, quenching protocol, *etc.*[4,5]

Figure S1-(a, c) displays the time evolution of the number of liquid molecules at in the pressure range from $p = 700$ atm to $p = 900$ atm for basal (a) and secondary prism (c) faces. As can be seen, the simulation time for the basal face is larger as compared to the secondary prism face. The fluctuations of the number of liquid molecules are also more pronounced in the former case. In Figure S1-(b, d) melting/freezing rates were plotted as a function of pressure and the melting pressure $p_m$ is located by interpolation to zero rate. The coexistence pressures are similar and are equal to $p_m = 807 \pm 0.87$ atm and $p_m = 797 \pm 0.68$ atm for basal and pII, respectively. Therefore, we have estimated the final melting pressure as an average equal to 802 atm. Error bars have been estimated separately for each case as $\Delta p_m = (\Delta a/a + \Delta b/b)p_m$ with $\Delta a, \Delta b$ being standard errors. Linear regressions in the form of $y = a + bx$ and standard errors are presented in insets to Fig. S1-(b,d).

## Validation of piston barostat

The pressure exerted by the wall on the fluid must be balanced by the corresponding force exerted by the fluid on the wall. It can be calculated as follows:[6]

$$p_z = \frac{1}{A} \sum_i f_z(\mathbf{r}_i) \tag{1}$$

where $f_z$ is the $z$ component of the force exerted by the wall on a water molecule at $(\mathbf{r}_i)$, and the sum runs over all water molecules within the cutoff distance from the wall.

An alternative, and more readily accessible option is to validate if the density in the middle of the slit is the same as in bulk under the same thermodynamic conditions. An example of such approach is shown in Figure S2. It is visible that the density in the middle of a slit fluctuates around a mean value corresponding to the bulk density at the same thermodynamic conditions.

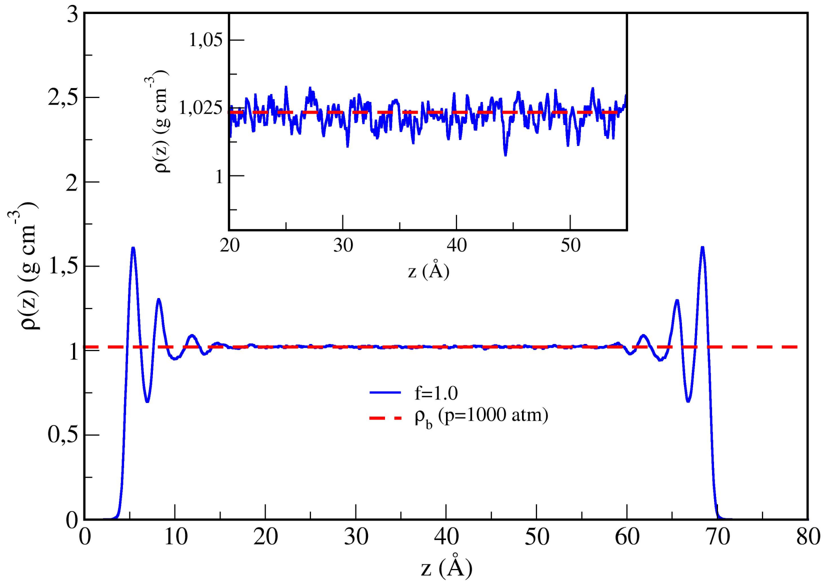


Figure S2: Density profile of a liquid water at $T$ = 262 K and $p$ = 1000 atm for the hydrophobic system with $f = 1/\theta = 120°$. The red dashed line corresponds to the bulk density at the same thermodynamic conditions.

## Calculation of the Hamaker constant

The Hamaker constant can be calculated using Equation 22 from the main text which can be cast as:

$$A = 4\pi^2 \varepsilon \sigma^6 \left( \sqrt{f} \rho_S - \rho_w \right) (\rho_i - \rho_w) \tag{2}$$

where $\epsilon$ and $\sigma$ are the Lennard-Jones parameters of the TIP4P/Ice water model, while $\rho_S$, $\rho_i$ and $\rho_w$ are the number densities of the model wall, ice and water, respectively and $f$ is the parameter dictating the hydrophilicity of the wall. The bulk water and ice densities can be found in Tables S1, S2 for an isotherm at $T = 262$ K and isobar at $p = 1$ atm. The wall's density can be evaluated from the ice's densities at specific thermodynamic condition, taken into account that it is smaller by a factor of $(3/4) \times \sqrt{2} \approx 0.53$.

Calculated Hamaker constants can be found in Table S3, S4 and are plotted in Figure S3.

**Table S1: Water and ice densities along an isotherm at $T = 262$ K.**

| $p$ (atm) | $\rho_{ice}$ (g/cm$^3$) | $\rho_{ice}$ (No. density) | $\rho_{liq}$ (g/cm$^3$) | $\rho_{liq}$ (No. density) | $\Delta\rho$ (No. density) |
|---|---|---|---|---|---|
| -2000 | 0.8875 | 0.02967 | 0.8786 | 0.02937 | -0.00030 |
| -1600 | 0.8911 | 0.2979 | 0.8932 | 0.02986 | 0.00007 |
| -1200 | 0.8949 | 0.02991 | 0.9093 | 0.03039 | 0.00048 |
| -1000 | 0.8966 | 0.02997 | 0.9179 | 0.03068 | 0.00071 |
| -800 | 0.8983 | 0.03003 | 0.9269 | 0.03098 | 0.00096 |
| -600 | 0.8999 | 0.03008 | 0.9354 | 0.03127 | 0.00119 |
| -400 | 0.9016 | 0.03014 | 0.9468 | 0.03165 | 0.00151 |
| -200 | 0.9033 | 0.03019 | 0.9577 | 0.03201 | 0.00182 |
| 0 | 0.9049 | 0.03025 | 0.9695 | 0.03241 | 0.00216 |
| 200 | 0.9066 | 0.03031 | 0.9806 | 0.03278 | 0.00247 |
| 400 | 0.9082 | 0.03036 | 0.9915 | 0.03314 | 0.00278 |
| 600 | 0.9098 | 0.03041 | 1.0029 | 0.03352 | 0.00311 |
| 700 | 0.9107 | 0.03044 | 1.0080 | 0.03369 | 0.00325 |
| 800 | 0.9114 | 0.03047 | 1.0132 | 0.03387 | 0.00340 |
| 850 | 0.9118 | 0.03048 | 1.0155 | 0.03394 | 0.00347 |
| 900 | 0.9123 | 0.03049 | 1.0178 | 0.03402 | 0.00353 |

**Table S2: Water and ice densities along an isobar at $p = 1$ atm.**

| $T$ (K) | $\rho_{ice}$ (g/cm$^3$) | $\rho_{ice}$ (No. density) | $\rho_{liq}$ (g/cm$^3$) | $\rho_{liq}$ (No. density) |
|---|---|---|---|---|
| 230 | 0.9095 | 0.03040 | 0.9298 | 0.03108 |
| 240 | 0.9081 | 0.03035 | 0.9412 | 0.03146 |
| 250 | 0.9067 | 0.03031 | 0.9574 | 0.03200 |
| 256 | 0.9059 | 0.03028 | 0.9619 | 0.03215 |
| 260 | 0.9053 | 0.03026 | 0.9680 | 0.03236 |
| 266 | 0.9045 | 0.03023 | 0.9715 | 0.03247 |
| 269 | 0.9041 | 0.03022 | 0.9736 | 0.03254 |
| 270 | 0.9039 | 0.03021 | 0.9743 | 0.03257 |

**Table S3: The Hamaker constant evaluated along an isobar at $p = 1$ atm.**

| $p$ (atm) | $A$ (zJ) | | | |
|---|---|---|---|---|
| | $f = 1$ | $f = 2$ | $f = 3$ | $f = 4$ |
| -2000 | | | | 0.0366 |
| -1600 | | | | -0.0072 |
| -1200 | | | 0.0820 | -0.0374 |
| -1000 | | | 0.1316 | -0.0460 |
| -800 | | 0.4720 | 0.1897 | -0.0483 |
| -600 | | 0.6031 | 0.2519 | -0.0441 |
| -400 | | 0.7956 | 0.3486 | -0.0282 |
| -200 | 1.6977 | 0.9940 | 0.4539 | -0.0013 |
| 0 | 2.0608 | 1.2241 | 0.5820 | 0.0410 |
| 200 | 2.4102 | 1.4498 | 0.7129 | 0.0916 |
| 400 | 2.7686 | 1.6853 | 0.8540 | 0.1532 |
| 600 | 3.1553 | 1.9434 | 1.0134 | 0.2295 |
| 700 | 3.3301 | 2.0613 | 1.0877 | 0.2669 |
| 800 | 3.5170 | 2.1882 | 1.1685 | 0.3089 |
| 850 | 3.5947 | 2.2411 | 1.2025 | 0.3269 |
| 900 | 3.6730 | 2.2946 | 1.2369 | 0.3453 |

**Table S4: The Hamaker constant evaluated along an isobar at $p = 1$ atm.**

| $T$ (K) | $A$ (zJ) | | | |
|---|---|---|---|---|
| | $f = 1$ | $f = 2$ | $f = 3$ | $f = 4$ |
| 230 | 0.5939 | 0.3288 | 0.1253 | -0.0462 |
| 240 | 0.9930 | 0.5620 | 0.2314 | -0.0474 |
| 250 | 1.5743 | 0.9163 | 0.4114 | -0.0142 |
| 256 | 1.7582 | 1.0315 | 0.4740 | 0.0040 |
| 260 | 1.9922 | 1.1800 | 0.5569 | 0.0316 |
| 262 | 2.0608 | 1.2241 | 0.5820 | 0.0408 |
| 266 | 2.1489 | 1.2808 | 0.6147 | 0.0532 |
| 269 | 2.1096 | 1.2556 | 0.6003 | 0.0479 |
| 270 | 2.2715 | 1.3602 | 0.6610 | 0.0715 |

**Table S5: The disjoining pressure and premelting film heights evaluated along an isobar at $p = 1$ atm.**

| $T$ (K) | $h$ (Å) | | | | $\Pi(h)$ (atm) |
|---|---|---|---|---|---|
| | $f = 1$ | $f = 2$ | $f = 3$ | $f = 4$ | |
| 230 | 3.234 | 3.132 | 6.032 | 4.485 | 324.61 |
| 240 | 4.713 | 4.741 | 6.955 | 4.971 | 264.66 |
| 250 | 5.375 | 5.718 | 8.868 | 9.053 | 189.23 |
| 256 | 5.745 | 6.252 | 8.964 | 10.189 | 137.63 |
| 260 | 6.656 | 7.676 | 9.292 | 11.175 | 99.86 |
| 262 | 8.456 | 8.793 | 10.505 | 12.447 | 77.39 |
| 266 | 8.929 | 10.066 | 13.451 | 14.124 | 41.49 |
| 269 | 9.610 | 14.860 | 17.185 | 19.961 | 10.05 |
| 270 | 19.736 | 25.428 | 23.654 | 26.962 | 0.0 |

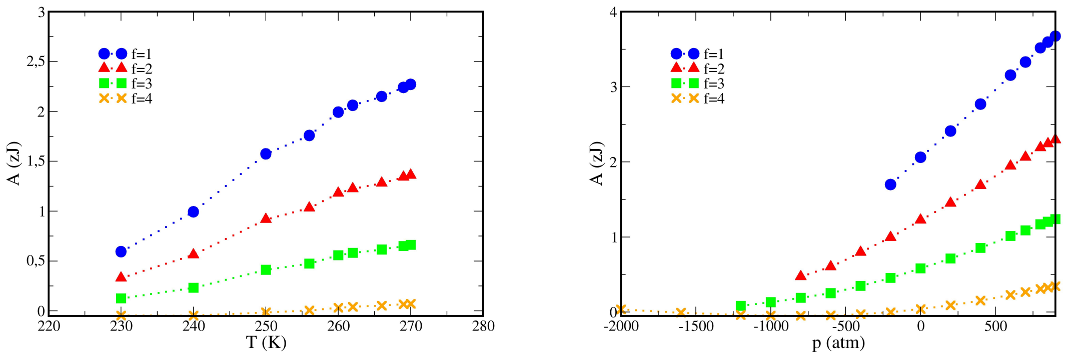


Figure S3: Hamaker constant evaluated along an isobar at $p = 1$ atm (left panel) and isotherm at $T = 262$ K (right panel).

**Table S6: The disjoining pressure and premelting film heights evaluated along an isotherm at $T = 262$ K.**

| $p$ (atm) | $h$ (Å) | | | | $\Pi(h)$ (atm) |
|---|---|---|---|---|---|
| | $f=1$ | $f=2$ | $f=3$ | $f=4$ | |
| -2000 | | | | 9.511 | 82.45 |
| -1600 | | | | 9.639 | 100.28 |
| -1200 | | | 9.013 | 9.556 | 109.26 |
| -1000 | | | 9.201 | 9.668 | 110.27 |
| -800 | | 4.863 | 9.144 | 9.488 | 108.86 |
| -600 | | 7.053 | 9.100 | 9.977 | 104.96 |
| -400 | | 6.861 | 9.360 | 11.791 | 98.48 |
| -200 | 6.476 | 8.467 | 10.573 | 10.791 | 89.34 |
| 0 | 8.456 | 8.793 | 10.505 | 12.447 | 77.39 |
| 200 | 8.576 | 8.857 | 12.047 | 12.408 | 62.72 |
| 400 | 8.856 | 10.349 | 14.552 | 13.819 | 45.04 |
| 600 | 9.590 | 13.273 | 14.856 | 15.308 | 24.30 |
| 700 | 9.996 | 13.146 | 15.577 | 17.110 | 12.74 |
| 800 | 16.662 | 16.476 | 19.341 | 19.032 | 0.38 |
| 850 | 20.393 | 19.743 | 18.620 | 18.034 | -6.10 |
| 900 | 17.589 | 19.203 | 24.866 | 22.154 | -12.80 |

# Equilibrim properties of the model interface potential

Our calculations support a minimal model of interface potential given by:

$$g(h) = Ce^{-\kappa h} - \frac{A}{12\pi h^2} \tag{3}$$

For our systems, $C$ is found to be positive, while $A$ is positive for contact angles greater than 50° and negative otherwise. In the former case, $g(h)$ exhibits a minimum, which may be found from the following equation:

$$\kappa h_e = -3W_{-1}\left(-\frac{1}{3}K^{1/3}\right) \tag{4}$$

where $W_{-1}(x)$ is the $-1$ branch of the Lambert $W$ function (also known as the Product-Log function) while:

$$K = \frac{A\kappa^2}{6\pi C} \tag{5}$$

For $A$ positive, $g(h)$ has also an inflection point which corresponds to a wetting spinodal that can also be of interest in some situations. The equation to locate the spinodal film thickness is:

$$\kappa h_{sp} = -4W_{-1}\left(-\frac{1}{4}(3K)^{1/4}\right) \tag{6}$$

As a word of caution notice that for very short film thicknesses, the model of Eq.3 also exhibits a spurious maximum at $\kappa h_m = -3W_0\left(-\frac{1}{3}K^{1/3}\right)$ and then diverges towards $-\infty$ as $h \to 0$. This part of the model is not meant to be physically significant. The problem is not really relevant, as this behavior occurs at film thicknesses of the order $\kappa h \approx K^{1/3}$, which are very small sub-angstrom scales that are never attained in practice in our systems.

# References


(1) García Fernández, R.; Abascal, J. L. F.; Vega, C. The melting point of ice Ih for common water models calculated from direct coexistence of the solid-liquid interface. *J. Chem. Phys.* **2006**, *124*, 144506.

(2) Ladd, A.; Woodcock, L. Interfacial and co-existence properties of the Lennard-Jones system at the triple point. *Molecular Physics* **1978**, *36*, 611–619.

(3) Nada, H.; Furukawa, Y. Anisotropy in Growth Kinetics at Interfaces Between Proton Disordered Hexagonal Ice and Water: A Molecular Dynamics Study Using the Six-Site Model of H2O. *J. Cryst. Growth* **2005**, *283*, 242.

(4) Lupi, L.; Hudait, A.; Peters, B.; Grünwald, M.; Mullen, R. G.; Nguyen, A. H.; Molinero, V. Role of Stacking Disorder in Ice Nucleation. *Nature* **2017**, *551*, 218–222.

(5) Pirzadeh, P.; Kusalik, P. G. On Understanding Stacking Fault Formation in Ice. *Journal of the American Chemical Society* **2011**, *133*, 704–707, PMID: 21190379.

(6) Baran, Ł.; Llombart, P.; Rżysko, W.; MacDowell, L. G. Ice Friction at the Nanoscale. *Proc. Natl. Acad. Sci. U.S.A.* **2022**, *119*, e2209545119.
